# Supplementary material for: Numerically Stable Resonating Hartree-Fock
Source: arXiv:2411.00712 ancillary file (2025-03-13)
Supplement: Supplementary file 1 [file supplement.pdf]

# Numerically Stable Resonating Hartree-Fock

Ericka Roy Miller and Shane M. Parker<sup>a)</sup>Department of Chemistry, Case Western Reserve University  
10900 Euclid Ave, Cleveland, OH 44106, USA

## I. SPIN EXPECTATION VALUES OF RESHF STATES

In the following derivation, we will use an adapted version of Fukutome's notation<sup>1</sup>, which deviates slightly from the notation of our main text. We define general spin MO creation and annihilation operators,

$$\hat{c}_p^\dagger|-\rangle = |\phi_p\rangle \text{ and } \hat{c}_q|\phi_p\rangle = |-\rangle, \quad (1)$$

which are associated with a reference Slater determinant. These second quantization operators observe the standard Fermionic anticommutation relationship

$$\{\hat{c}_p^\dagger, \hat{c}_q\} = \delta_{pq}. \quad (2)$$

We can apply Thouless transformations to generate a set of nonorthogonal Slater determinants from this reference. Fukutome then showed that the one-body reduced density matrix can be derived in the spin MO representation as

$$Q_{qp}^{AB} = \sum_{ij} B_{qi}(S_{ji}^{AB})^{-1} A_{jp}^* \quad (3)$$

$$\langle \Phi_A | \hat{c}_p^\dagger \hat{c}_q | \Phi_B \rangle = \langle \Phi_A | \Phi_B \rangle Q_{qp}^{AB} = \gamma_{qp}^{AB}, \quad (4)$$

where  $B_{qi}$  and  $A_{jp}^*$  represent Thouless transformations from the reference Slater determinant. The two-body reduced density matrix in the spin MO representation is

$$\langle \Phi_A | \hat{c}_p^\dagger \hat{c}_q^\dagger \hat{c}_s \hat{c}_r | \Phi_B \rangle = \langle \Phi_A | \Phi_B \rangle (Q_{rp}^{AB} Q_{sq}^{AB} - Q_{rq}^{AB} Q_{sp}^{AB}). \quad (5)$$

For clarity, we define an alternative notation for our spin MO creation and annihilation operators in order to more easily distinguish between  $\alpha$  and  $\beta$  spin orbitals:

$$\hat{p}_\alpha^\dagger|-\rangle = |\phi_p^\alpha\rangle \text{ and } \hat{q}_\beta|\phi_q^\beta\rangle = |-\rangle. \quad (6)$$

The spin contamination of a ResHF electronic state can be quantified by computing

$$\langle \Psi_I | \hat{S}^2 | \Psi_I \rangle = \sum_{AB} c_{IA}^* \langle \Phi_A | \hat{S}^2 | \Phi_B \rangle c_{BI}. \quad (7)$$

To compute  $\langle \Phi_A | \hat{S}^2 | \Phi_B \rangle$ , we will use

$$\hat{S}^2 = \hat{S}_z^2 - \hbar \hat{S}_z + \hat{S}_+ \hat{S}_-, \quad (8)$$

where the raising and lowering operators are

$$\hat{S}_\pm = \hat{S}_x \pm i \hat{S}_y. \quad (9)$$

In second quantization, the raising and lowering operators are

$$\hat{S}_+ = \sum_p \hat{p}_\alpha^\dagger \hat{p}_\beta \quad (10)$$

$$\hat{S}_- = \sum_p \hat{p}_\beta^\dagger \hat{p}_\alpha. \quad (11)$$

<sup>a)</sup>Electronic mail: shane.parker@case.edu

Thus,

$$\hat{S}_+ \hat{S}_- = \sum_{pq} \hat{p}_\alpha^\dagger \hat{p}_\beta \hat{q}_\beta^\dagger \hat{q}_\alpha = \sum_{pq} \hat{p}_\alpha^\dagger (\delta_{pq} - \hat{q}_\beta^\dagger \hat{p}_\beta) \hat{q}_\alpha = \sum_p \hat{p}_\alpha^\dagger \hat{p}_\alpha - \sum_{pq} \hat{p}_\alpha^\dagger \hat{q}_\beta^\dagger \hat{p}_\beta \hat{q}_\alpha = \hat{n}_\alpha - \sum_{pq} \hat{p}_\alpha^\dagger \hat{q}_\beta^\dagger \hat{p}_\beta \hat{q}_\alpha. \quad (12)$$

Thus, the final operator expression used for  $\langle \Phi_A | \hat{S}^2 | \Phi_B \rangle$  expectation values will be

$$\hat{S}^2 = \hat{S}_z^2 - \hbar \hat{S}_z + \hat{n}_\alpha - \sum_{pq} \hat{p}_\alpha^\dagger \hat{q}_\beta^\dagger \hat{p}_\beta \hat{q}_\alpha. \quad (13)$$

The first three terms are straightforward to compute because we use unrestricted orbitals, which are eigenfunctions of  $\hat{S}_z$  and  $\hat{n}_\alpha$ :

$$\langle \Phi_A | \hat{S}_z^2 - \hbar \hat{S}_z + \hat{n}_\alpha | \Phi_B \rangle = \left( \frac{1}{4} (n_\alpha - n_\beta)^2 - \frac{1}{2} (n_\alpha - n_\beta) + n_\alpha \right) \langle \Phi_A | \Phi_B \rangle. \quad (14)$$

For the last term, we use Eq. (5) to find

$$\sum_{pq} \langle \Phi_A | \hat{p}_\alpha^\dagger \hat{q}_\beta^\dagger \hat{p}_\beta \hat{q}_\alpha | \Phi_B \rangle = \langle \Phi_A | \Phi_B \rangle \sum_{pq} (Q_{q_\alpha p_\alpha}^{AB} Q_{p_\beta q_\beta}^{AB} - Q_{q_\alpha q_\beta}^{AB} Q_{p_\beta p_\alpha}^{AB}) \quad (15a)$$

$$= \langle \Phi_A | \Phi_B \rangle \langle \mathbf{Q}^{AB,\alpha} \mathbf{Q}^{AB,\beta} \rangle, \quad (15b)$$

where  $\langle \cdot \rangle$  is the matrix trace. Putting it all together, we have

$$\langle \Psi_I | \hat{S}^2 | \Psi_I \rangle = \sum_{AB} c_{AI}^* \langle \Phi_A | \hat{S}^2 | \Phi_B \rangle c_{BI} \quad (16)$$

$$\langle \Phi_A | \hat{S}^2 | \Phi_B \rangle = \left( \frac{1}{4} (n_\alpha - n_\beta)^2 - \frac{1}{2} (n_\alpha - n_\beta) + n_\alpha \right) \langle \Phi_A | \Phi_B \rangle - \langle \mathbf{Q}^{AB,\alpha} \mathbf{Q}^{AB,\beta} \rangle \langle \Phi_A | \Phi_B \rangle. \quad (17)$$

## II. 4SA-RESHF AND 4SA-CASSCF VERTICAL EXCITATION ENERGIES

TABLE SI: Vertical excitation energies (in eV) for selected QUEST database molecules. 4SA-CASSCF(2e,2o) and 4SA-ResHF(4sd) energies were computed using the def2-QZVP basis set.  $\langle S^2 \rangle$  values for ResHF states are shown in parentheses. Theoretical best estimates (TBE) obtained from QUEST are used to compute mean average errors (MAE). Singlet-triplet energy gaps are calculated as  $\Delta E_{st} = E_{S_1} - E_{T_1}$ .

| Molecule          | 4SA-CASSCF |           |                 | 4SA-ResHF    |              |                 | TBE       |           |                   |
|-------------------|------------|-----------|-----------------|--------------|--------------|-----------------|-----------|-----------|-------------------|
|                   | $E_{S_1}$  | $E_{T_1}$ | $\Delta E_{st}$ | $E_{S_1}$    | $E_{T_1}$    | $\Delta E_{st}$ | $E_{S_1}$ | $E_{T_1}$ | $\Delta E_{st}$   |
| formaldehyde      | 3.50       | 2.81      | 0.69            | 2.76 (0.064) | 2.41 (2.000) | 0.35            | 3.97      | 3.58      | 0.39 <sup>a</sup> |
| acetaldehyde      | 3.89       | 3.24      | 0.65            | 3.13 (0.067) | 2.81 (2.000) | 0.32            | 4.31      | 3.98      | 0.33 <sup>a</sup> |
| formamide         | 4.85       | 4.30      | 0.55            | 4.38 (0.055) | 4.13 (2.000) | 0.26            | 5.63      | 5.37      | 0.26 <sup>a</sup> |
| streptocyanine-C1 | 8.20       | 5.10      | 3.10            | 7.44 (0.093) | 5.87 (2.001) | 1.58            | 7.12      | 5.52      | 1.60 <sup>a</sup> |
| acetone           | 4.09       | 3.47      | 0.62            | 3.32 (0.066) | 3.02 (2.000) | 0.30            | 4.48      | 4.15      | 0.33 <sup>b</sup> |
| cyclopentadiene   | 6.38       | 3.47      | 2.91            | 6.21 (0.027) | 3.58 (2.000) | 2.63            | 5.55      | 3.31      | 2.24 <sup>b</sup> |
| pyrimidine        | 5.30       | 4.89      | 0.41            | —            | —            | —               | 4.45      | 4.10      | 0.35 <sup>b</sup> |
| benzoxadiazole    | 5.62       | 2.96      | 2.67            | —            | —            | —               | 4.52      | 2.74      | 1.78 <sup>c</sup> |
| benzothiadiazole  | 5.40       | 2.95      | 2.45            | —            | —            | —               | 4.23      | 2.82      | 1.41 <sup>c</sup> |
| MAE               | 0.79       | 0.55      | 0.60            | 0.96         | 0.89         | 0.08            |           |           |                   |

<sup>a</sup> Theoretical best estimates (TBE) taken from QUEST subset #1 (Ref. 2)

<sup>b</sup> Theoretical best estimates (TBE) taken from QUEST subset #3 (Ref. 3)

<sup>c</sup> Theoretical best estimates (TBE) taken from QUEST subset #7 (Ref. 4)

<sup>1</sup>H. Fukutome, “Theory of Resonating Quantum Fluctuations in a Fermion System: Resonating Hartree-Fock Approximation,” Prog. Theor. Phys. **80**, 417–432 (1988).

<sup>2</sup>P.-F. Loos, A. Scemama, A. Blondel, Y. Garniron, M. Caffarel, and D. Jacquemin, “A mountaineering strategy to excited states: Highly accurate reference energies and benchmarks,” J. Chem. Theory Comput. **14**, 4360–4379 (2018).

<sup>3</sup>P.-F. Loos, F. Lipparini, M. Boggio-Pasqua, A. Scemama, and D. Jacquemin, “A mountaineering strategy to excited states: Highly accurate energies and benchmarks for medium sized molecules,” J. Chem. Theory Comput. **16**, 1711–1741 (2020).

<sup>4</sup>P.-F. Loos and D. Jacquemin, “A mountaineering strategy to excited states: Highly accurate energies and benchmarks for bicyclic systems,” J. Phys. Chem. A **125**, 10174–10188 (2021).
